# Supplementary material for: The Broad Absorption Line Tidal Disruption Event iPTF15af: Optical and Ultraviolet Evolution
Source: arXiv:1809.07446 source file (2020-06-25)
Supplement: Supplementary file 1 [file supplementary.tex]

\begin{deluxetable*}{rrcccccccccc} 
\tabletypesize{\scriptsize} 
\tablewidth{0pt} 
\tablecaption{Optical difference imaging and \textit{Swift} UV aperture photometry of iPTF15af in AB magnitude system. \\
The $r$-band column for the P48 contains measurements in Mould-$R$ filter system.\\
These measurements are not corrected for Galactic extinction. Table \ref{table:phot} is published in its entirety in the machine-readable format. A portion is shown here for guidance regarding its form and content. \label{table:phot}} 
\tablehead{ 
   \colhead{MJD}     &  \colhead{Phase}     &\colhead{Telescope + Instrument}    &  \colhead{$UVW1$} &  \colhead{$UVM2$} &  \colhead{$UVW2$} &  \colhead{$U$} &  \colhead{$B$} &  \colhead{$V$} &  \colhead{$g$} &  \colhead{$r$} &  \colhead{$i$} \\ 
\colhead{ (days) } &  \colhead{ (days) }&  \colhead{(mag)}&  \colhead{(mag)}&  \colhead{(mag)}&  \colhead{(mag)}&  \colhead{(mag)}&  \colhead{(mag)}&  \colhead{(mag)}&  \colhead{(mag)}&  \colhead{(mag)}\\ \hline
} 
\startdata 
 56664.0 & $-$373.3 & PTFP48 & -- & -- & -- & -- & -- & -- & -- & $>$23.29 & --\\
 56667.0 & $-$370.3 & PTFP48 & -- & -- & -- & -- & -- & -- & -- & $>$22.20 & --\\
 56670.0 & $-$367.3 & PTFP48 & -- & -- & -- & -- & -- & -- & -- & $>$20.47 & --\\
 56769.0 & $-$268.3 & PTFP48 & -- & -- & -- & -- & -- & -- & -- & $>$21.89 & --\\
 57012.0 & $-$25.3 & PTFP48 & -- & -- & -- & -- & -- & -- & -- & 21.79$\pm$0.26 & --\\
 57015.0 & $-$22.3 & PTFP48 & -- & -- & -- & -- & -- & -- & -- & 21.73$\pm$0.12 & --\\
 57018.0 & $-$19.3 & PTFP48 & -- & -- & -- & -- & -- & -- & -- & 21.51$\pm$0.16 & --\\
 57021.0 & $-$16.3 & PTFP48 & -- & -- & -- & -- & -- & -- & -- & 21.51$\pm$0.18 & --\\
 57036.0 & $-$1.3 & PTFP48 & -- & -- & -- & -- & -- & -- & -- & 20.87$\pm$0.11 & --\\
 57039.3 & 2.0 & P60+SEDM & -- & -- & -- & -- & -- & -- & 20.27$\pm$0.06 & 20.58$\pm$0.10 & 20.55$\pm$0.14\\
 57039.0 & 1.7 & PTFP48 & -- & -- & -- & -- & -- & -- & -- & 20.64$\pm$0.05 & --\\
 57044.3 & 7.0 & P60+SEDM & -- & -- & -- & -- & -- & -- & 20.13$\pm$0.07 & 20.20$\pm$0.12 & $>$20.20\\
 57045.0 & 7.7 & PTFP48 & -- & -- & -- & -- & -- & -- & -- & 20.48$\pm$0.07 & --\\
 57045.2 & 7.9 & Las Cumbres 1m & -- & -- & -- & -- & 20.58$\pm$0.28 & 20.50$\pm$0.29 & 20.10$\pm$0.16 & 20.38$\pm$0.16 & 19.83$\pm$0.27\\
 57048.0 & 10.7 & PTFP48 & -- & -- & -- & -- & -- & -- & -- & 20.48$\pm$0.09 & --\\
 57049.2 & 11.9 & Swift+UVOT & 19.42$\pm$0.09 & 19.20$\pm$0.07 & 18.98$\pm$0.06 & 19.65$\pm$0.20 & 18.92$\pm$0.20 & 18.03$\pm$0.21 & -- & -- & --\\
 57050.4 & 13.1 & Las Cumbres 1m & -- & -- & -- & -- & 20.39$\pm$0.22 & 20.20$\pm$0.15 & 20.09$\pm$0.17 & 20.69$\pm$0.26 & 20.22$\pm$0.29\\
 57052.5 & 15.2 & Las Cumbres 1m & -- & -- & -- & -- & 19.82$\pm$0.43 & 20.00$\pm$0.41 & 19.76$\pm$0.18 & 20.59$\pm$0.40 & 19.91$\pm$0.30\\
 57053.5 & 16.2 & Swift+UVOT & 19.33$\pm$0.09 & 19.17$\pm$0.06 & 18.95$\pm$0.06 & 19.52$\pm$0.16 & 18.87$\pm$0.18 & 17.95$\pm$0.18 & -- & -- & --\\
 57059.8 & 22.5 & Swift+UVOT & 19.10$\pm$0.09 & 19.10$\pm$0.08 & 18.88$\pm$0.07 & 19.11$\pm$0.16 & 18.40$\pm$0.17 & 17.58$\pm$0.18 & -- & -- & --\\
 57062.2 & 24.9 & Las Cumbres 1m & -- & -- & -- & -- & -- & 20.18$\pm$0.20 & 19.85$\pm$0.28 & 20.51$\pm$0.24 & --\\
 57063.1 & 25.8 & P60+SEDM & -- & -- & -- & -- & -- & -- & -- & -- & 20.29$\pm$0.11\\
 57062.6 & 25.3 & Las Cumbres 1m & -- & -- & -- & -- & 19.67$\pm$0.72 & -- & -- & -- & --\\
 57063.8 & 26.5 & P60+SEDM & -- & -- & -- & -- & -- & -- & 19.89$\pm$0.07 & 20.18$\pm$0.08 & $>$21.10\\
 57064.3 & 27.0 & Swift+UVOT & 19.30$\pm$0.09 & 19.16$\pm$0.08 & 18.90$\pm$0.07 & 19.23$\pm$0.15 & 18.62$\pm$0.18 & 18.29$\pm$0.31 & -- & -- & --\\
 57067.1 & 29.8 & Las Cumbres 1m & -- & -- & -- & -- & 20.24$\pm$0.45 & 20.14$\pm$0.43 & 19.94$\pm$0.16 & 20.55$\pm$0.16 & 19.86$\pm$0.18\\
 57069.6 & 32.3 & Swift+UVOT & 19.36$\pm$0.08 & 19.16$\pm$0.06 & 18.92$\pm$0.05 & 19.23$\pm$0.13 & 18.83$\pm$0.16 & 17.90$\pm$0.16 & -- & -- & --\\
 57071.2 & 33.9 & P60+SEDM & -- & -- & -- & -- & -- & -- & 19.93$\pm$0.05 & 20.13$\pm$0.07 & 20.42$\pm$0.12\\
 57071.9 & 34.6 & Las Cumbres 1m & -- & -- & -- & -- & 19.57$\pm$0.47 & 20.32$\pm$0.41 & 19.94$\pm$0.17 & 20.54$\pm$0.34 & 19.84$\pm$0.23\\
 57073.8 & 36.5 & Las Cumbres 1m & -- & -- & -- & -- & 20.85$\pm$0.50 & -- & 19.76$\pm$0.22 & -- & --\\
 57074.8 & 37.5 & Swift+UVOT & 19.45$\pm$0.15 & 19.23$\pm$0.10 & 19.08$\pm$0.09 & 19.18$\pm$0.24 & 19.01$\pm$0.38 & 18.19$\pm$0.39 & -- & -- & --\\
 57078.2 & 40.9 & P60+SEDM & -- & -- & -- & -- & -- & -- & 19.78$\pm$0.07 & -- & --\\
 57078.3 & 41.0 & Las Cumbres 1m & -- & -- & -- & -- & 20.20$\pm$0.43 & 20.35$\pm$0.41 & 19.71$\pm$0.36 & -- & --\\
 57078.7 & 41.4 & P60+SEDM & -- & -- & -- & -- & -- & -- & -- & 20.24$\pm$0.16 & 20.27$\pm$0.17\\
 57079.2 & 41.9 & Swift+UVOT & 19.45$\pm$0.10 & 19.24$\pm$0.07 & 19.14$\pm$0.07 & 19.11$\pm$0.15 & 19.14$\pm$0.26 & 18.06$\pm$0.23 & -- & -- & --\\
 57078.9 & 41.6 & Las Cumbres 1m & -- & -- & -- & -- & -- & -- & -- & 20.34$\pm$0.17 & 19.90$\pm$0.25\\
 57080.2 & 42.9 & P60+SEDM & -- & -- & -- & -- & -- & -- & -- & 20.20$\pm$0.10 & 20.14$\pm$0.17\\
 57085.4 & 48.1 & Las Cumbres 1m & -- & -- & -- & -- & 20.52$\pm$0.39 & 20.06$\pm$0.55 & 19.91$\pm$0.14 & 20.65$\pm$0.27 & 19.83$\pm$0.34\\
 57086.8 & 49.5 & Las Cumbres 1m & -- & -- & -- & -- & -- & -- & 19.87$\pm$0.11 & -- & 20.31$\pm$0.25\\
 57089.3 & 52.0 & Swift+UVOT & 19.48$\pm$0.09 & 19.42$\pm$0.07 & 19.16$\pm$0.06 & 19.27$\pm$0.13 & 18.81$\pm$0.16 & 17.91$\pm$0.17 & -- & -- & --\\
 57091.2 & 53.9 & P60+SEDM & -- & -- & -- & -- & -- & -- & 20.09$\pm$0.05 & 20.39$\pm$0.08 & --\\
 57094.1 & 56.8 & P60+SEDM & -- & -- & -- & -- & -- & -- & 20.06$\pm$0.07 & 20.26$\pm$0.13 & --\\
 57094.0 & 56.7 & Las Cumbres 1m & -- & -- & -- & -- & -- & 20.42$\pm$0.57 & 20.10$\pm$0.12 & 20.76$\pm$0.24 & 20.10$\pm$0.26\\
 57095.4 & 58.1 & Las Cumbres 1m & -- & -- & -- & -- & 20.96$\pm$0.18 & -- & -- & -- & --\\
 57096.2 & 58.9 & P60+SEDM & -- & -- & -- & -- & -- & -- & 20.11$\pm$0.10 & 20.35$\pm$0.17 & --\\
 57095.7 & 58.4 & Las Cumbres 1m & -- & -- & -- & -- & -- & -- & -- & 20.77$\pm$0.49 & 19.98$\pm$0.36\\
 57098.1 & 60.8 & P60+SEDM & -- & -- & -- & -- & -- & -- & $>$18.40 & $>$18.50 & --\\
 57100.2 & 62.9 & P60+SEDM & -- & -- & -- & -- & -- & -- & 19.98$\pm$0.07 & 20.28$\pm$0.12 & --\\
 57099.6 & 62.3 & Swift+UVOT & 19.71$\pm$0.10 & 19.59$\pm$0.07 & 19.35$\pm$0.07 & 19.44$\pm$0.15 & 18.92$\pm$0.18 & 18.17$\pm$0.21 & -- & -- & --\\
 57101.8 & 64.5 & Las Cumbres 1m & -- & -- & -- & -- & 19.57$\pm$0.51 & 20.82$\pm$0.58 & 20.15$\pm$0.15 & -- & 20.31$\pm$0.25\\
 57103.1 & 65.8 & P60+SEDM & -- & -- & -- & -- & -- & -- & 20.09$\pm$0.04 & 20.31$\pm$0.08 & --\\
 57108.2 & 70.9 & P60+SEDM & -- & -- & -- & -- & -- & -- & 20.29$\pm$0.05 & 20.68$\pm$0.05 & --\\
 57108.0 & 70.7 & Las Cumbres 1m & -- & -- & -- & -- & -- & 20.23$\pm$0.38 & 20.14$\pm$0.16 & 20.92$\pm$0.41 & 20.07$\pm$0.26\\
 57108.6 & 71.3 & Swift+UVOT & 19.72$\pm$0.10 & 19.64$\pm$0.07 & 19.54$\pm$0.07 & 19.65$\pm$0.19 & 18.62$\pm$0.15 & 18.05$\pm$0.19 & -- & -- & --\\
 57114.1 & 76.8 & P60+SEDM & -- & -- & -- & -- & -- & -- & $>$20.20 & $>$20.30 & --\\
 57119.0 & 81.7 & Las Cumbres 1m & -- & -- & -- & -- & 20.99$\pm$0.30 & 20.90$\pm$0.26 & 20.41$\pm$0.30 & -- & 19.86$\pm$0.26\\
 57124.7 & 87.4 & Las Cumbres 1m & -- & -- & -- & -- & 20.84$\pm$0.44 & 21.16$\pm$0.35 & 20.27$\pm$0.15 & 20.77$\pm$0.29 & 20.33$\pm$0.22\\
 57154.2 & 116.9 & P60+SEDM & -- & -- & -- & -- & -- & -- & $>$21.00 & $>$20.40 & --\\
 57168.2 & 130.9 & P60+SEDM & -- & -- & -- & -- & -- & -- & $>$20.80 & $>$20.60 & --\\
 57168.3 & 131.0 & Swift+UVOT & 20.06$\pm$0.12 & 20.46$\pm$0.09 & 20.34$\pm$0.09 & 19.90$\pm$0.28 & 18.74$\pm$0.21 & 18.21$\pm$0.26 & -- & -- & --\\
 57171.2 & 133.9 & P60+SEDM & -- & -- & -- & -- & -- & -- & $>$21.10 & $>$21.30 & --\\
 57174.2 & 136.9 & P60+SEDM & -- & -- & -- & -- & -- & -- & -- & $>$21.00 & --\\
 57177.4 & 140.1 & Swift+UVOT & $>$20.78 & 20.40$\pm$0.15 & 20.41$\pm$0.16 & $>$19.54 & $>$18.70 & $>$17.81 & -- & -- & --\\
 57185.3 & 148.0 & Swift+UVOT & 20.44$\pm$0.21 & 20.40$\pm$0.11 & 20.25$\pm$0.10 & 19.53$\pm$0.30 & 18.72$\pm$0.30 & $>$18.11 & -- & -- & --\\
 \enddata 
\end{deluxetable*}
